# Supplementary material for: Accelerating QM/MM simulations of electrochemical interfaces through machine learning of electronic charge densities
Source: arXiv:2405.07370 ancillary file (2024-05-12)
Supplement: Supplementary file 1 [file suppl_mat.pdf]

# Accelerating QM/MM simulations of electrochemical interfaces through machine learning of electronic charge densities - Supplementary Material

Andrea Grisafi<sup>1,\*</sup> and Mathieu Salanne<sup>2,3,†</sup>

<sup>1</sup>*Institut Sciences du Calcul et des Données, ISCD, Sorbonne Université, F-75005 Paris, France*

<sup>2</sup>*Physicochimie des Électrolytes et Nanosystèmes Interfaciaux,  
Sorbonne Université, CNRS, F-75005 Paris, France*

<sup>3</sup>*Institut Universitaire de France (IUF), F-75231 Paris, France*

# DERIVATION OF HARTREE POTENTIAL AND ELECTRIC FIELD IN REAL SPACE

Let us consider the Hartree potential that can be derived from the linear atom-centered expansion of the electron density  $n_e$  of a non-periodic system:

$$\begin{aligned}\phi_H(\mathbf{r}) &= \int_{\mathbf{R}^3} d\mathbf{r}' \frac{n_e(\mathbf{r}')}{|\mathbf{r} - \mathbf{r}'|} \\ &= \sum_{i=1}^N \sum_{nlm} c_i^{nlm} \int_{\mathbf{R}^3} d\mathbf{r}' \frac{R_n^l(|\mathbf{r}' - \mathbf{r}_i|) Y_m^l(\widehat{\mathbf{r}' - \mathbf{r}_i})}{|\mathbf{r} - \mathbf{r}'|} \\ &= \sum_{i=1}^N \sum_{nlm} c_i^{nlm} \int_{\mathbf{R}^3} d\mathbf{s} \frac{R_n^l(s) Y_m^l(\widehat{\mathbf{s}})}{|(\mathbf{r} - \mathbf{r}_i) - \mathbf{s}|}\end{aligned}\tag{S1}$$

where we adopted the change of variable  $\mathbf{s} = \mathbf{r}' - \mathbf{r}_i$  in the last equality. We now introduce a rotation of the reference frame in such a way that the vector  $\mathbf{r} - \mathbf{r}_i$  is aligned along  $\hat{\mathbf{z}}$ . Upon this transformation, the spherical harmonics undergo a passive rotation that is expressed by the proper Wigner-D matrix:

$$\phi_H(\mathbf{r}) = \sum_{i=1}^N \sum_{nlm} c_i^{nlm} \sum_{m'} D_{mm'}^{l\dagger}(\widehat{\mathbf{r} - \mathbf{r}_i} \rightarrow \hat{\mathbf{z}}) \int_{\mathbf{R}^3} d\mathbf{s} \frac{R_n^l(s) Y_{m'}^l(\widehat{\mathbf{s}})}{|(\mathbf{r} - \mathbf{r}_i) - \mathbf{s}|},\tag{S2}$$

where now  $\hat{\mathbf{z}} \parallel \widehat{\mathbf{r} - \mathbf{r}_i}$  within the integral. This alignment allows us to make use of spherical coordinates to express the orientation of  $\mathbf{s}$  with respect to  $\mathbf{r} - \mathbf{r}_i$ , so that we can write

$$|(\mathbf{r} - \mathbf{r}_i) - \mathbf{s}| = \sqrt{|\mathbf{r} - \mathbf{r}_i|^2 + s^2 - 2|\mathbf{r} - \mathbf{r}_i|s \cos \theta}.\tag{S3}$$

From the symmetry of the Coulomb potential about the azimuthal angle  $\psi$ , performing the integral over  $\psi$  implies that only the components for which  $m' = 0$  survive:

$$\begin{aligned}\int_0^{2\pi} d\psi Y_{m'}^l(\theta, \psi) &= (-1)^{m'} \sqrt{\frac{2l+1}{4\pi} \frac{(l-m')!}{(l+m')!}} P_l(\cos \theta) \int_0^{2\pi} d\psi e^{im'\psi} \\ &= \sqrt{\frac{2l+1}{4\pi}} P_l(\cos \theta) 2\pi \delta_{m'0}.\end{aligned}\tag{S4}$$

Considering that,

$$D_{m0}^{l\dagger}(\widehat{\mathbf{r} - \mathbf{r}_i} \rightarrow \hat{\mathbf{z}}) = D_{0m}^l(\widehat{\mathbf{r} - \mathbf{r}_i} \rightarrow \hat{\mathbf{z}}) = \sqrt{\frac{4\pi}{2l+1}} Y_m^l(\widehat{\mathbf{r} - \mathbf{r}_i}),\tag{S5}$$

we are left with the following expression:

$$\begin{aligned}\phi_H(\mathbf{r}) &= 2\pi \sum_{i=1}^N \sum_{nlm} c_i^{nlm} Y_m^l(\widehat{\mathbf{r} - \mathbf{r}_i}) \\ &\quad \int_0^\infty ds s^2 R_n^l(s) \int_{-1}^1 d\cos \theta \frac{P_l(\cos \theta)}{\sqrt{|\mathbf{r} - \mathbf{r}_i|^2 + s^2 - 2|\mathbf{r} - \mathbf{r}_i|s \cos \theta}}.\end{aligned}\tag{S6}$$

At this point, we introduce the Laplace expansion of the Coulomb potential, i.e.,

$$(|\mathbf{r} - \mathbf{r}_i|^2 + s^2 - 2|\mathbf{r} - \mathbf{r}_i|s \cos \theta)^{-\frac{1}{2}} = \begin{cases} \sum_l \frac{s^l}{|\mathbf{r} - \mathbf{r}_i|^{l+1}} P_l(\cos \theta) & \text{for } s < |\mathbf{r} - \mathbf{r}_i| \\ \sum_l \frac{|\mathbf{r} - \mathbf{r}_i|^l}{s^{l+1}} P_l(\cos \theta) & \text{for } s > |\mathbf{r} - \mathbf{r}_i| \end{cases}\tag{S7}$$

The orthogonality of Legendre polynomials can finally be exploited to obtain

$$\begin{aligned}
\phi_H(\mathbf{r}) &= 2\pi \sum_{i=1}^N \sum_{nlm} c_i^{nlm} Y_m^l(\widehat{\mathbf{r} - \mathbf{r}_i}) \\
&\quad \frac{2}{2l+1} \left( \frac{1}{|\mathbf{r} - \mathbf{r}_i|^{l+1}} \int_0^{|\mathbf{r} - \mathbf{r}_i|} ds s^{2+l} R_n^l(s) + |\mathbf{r} - \mathbf{r}_i|^l \int_{|\mathbf{r} - \mathbf{r}_i|}^{\infty} ds s^{1-l} R_n^l(s) \right) \\
&= 4\pi \sum_{i=1}^N \sum_{nlm} c_i^{nlm} \frac{1}{2l+1} \left( \frac{I_{ln}^<(|\mathbf{r} - \mathbf{r}_i|)}{|\mathbf{r} - \mathbf{r}_i|^{l+1}} + |\mathbf{r} - \mathbf{r}_i|^l I_{ln}^>(|\mathbf{r} - \mathbf{r}_i|) \right) Y_m^l(\widehat{\mathbf{r} - \mathbf{r}_i})
\end{aligned} \tag{S8}$$

where  $I_{ln}^<$  and  $I_{ln}^>$  are the radial integrals.

### Electric field calculation

To analytically compute the electric field, it is convenient to express the Cartesian gradient in spherical coordinates:

$$\nabla = \mathbf{U} \cdot \tilde{\nabla}, \tag{S9}$$

where

$$\tilde{\nabla} \equiv \left( \frac{\partial}{\partial r}, \frac{1}{r} \frac{\partial}{\partial \theta}, \frac{1}{r \sin \theta} \frac{\partial}{\partial \phi} \right)$$

is the gradient in spherical coordinates, and where the matrix

$$\mathbf{U} = \begin{pmatrix} \sin \theta \cos \phi & \cos \theta \cos \phi & -\sin \phi \\ \sin \theta \sin \phi & \cos \theta \sin \phi & \cos \phi \\ \cos \theta & -\sin \theta & 0 \end{pmatrix}, \tag{S10}$$

represents the transformation between the unit vectors  $(\hat{x}, \hat{y}, \hat{z}) \rightarrow (\hat{r}, \hat{\theta}, \hat{\phi})$ . In particular, we can apply the substitution  $\mathbf{r} - \mathbf{r}_i \equiv (r, \theta, \phi)$  within the sum over atoms in Eq. (S8), and make use of the gradient in spherical coordinates to analytically work out the expression for the Hartree electric field:

$$\begin{aligned}
\mathbf{E}_H(\mathbf{r}) &= -\nabla \phi_H(\mathbf{r}) \\
&= -4\pi \sum_{i=1}^N \mathbf{U}(\mathbf{r} - \mathbf{r}_i) \sum_{nlm} \frac{c_i^{nlm}}{2l+1} \\
&\quad \left[ \frac{\partial}{\partial r} \left( \frac{1}{r^{l+1}} \int_0^r ds s^{2+l} R_n^l(s) + r^l \int_r^\infty ds s^{1-l} R_n^l(s) \right) Y_m^l(\theta, \phi), \right. \\
&\quad \left( \frac{1}{r^{l+1}} \int_0^r ds s^{2+l} R_n^l(s) + r^l \int_r^\infty ds s^{1-l} R_n^l(s) \right) \frac{1}{r} \frac{\partial}{\partial \theta} Y_m^l(\theta, \phi), \\
&\quad \left. \left( \frac{1}{r^{l+1}} \int_0^r ds s^{2+l} R_n^l(s) + r^l \int_r^\infty ds s^{1-l} R_n^l(s) \right) \frac{1}{r \sin \theta} \frac{\partial}{\partial \phi} Y_m^l(\theta, \phi) \right] \\
&= -4\pi \sum_{i=1}^N \mathbf{U}(\mathbf{r} - \mathbf{r}_i) \sum_{nlm} \frac{c_i^{nlm}}{2l+1} \\
&\quad \left[ \left( -\frac{l+1}{r^{l+2}} I_{ln}^<(r) + l r^{l-1} I_{ln}^>(r) \right) Y_m^l(\theta, \phi), \right. \\
&\quad \left( \frac{1}{r^{l+2}} I_{ln}^<(r) + r^{l-1} I_{ln}^>(r) \right) \frac{\partial}{\partial \theta} Y_m^l(\theta, \phi), \\
&\quad \left. \left( \frac{1}{r^{l+2}} I_{ln}^<(r) + r^{l-1} I_{ln}^>(r) \right) \frac{1}{\sin \theta} \frac{\partial}{\partial \phi} Y_m^l(\theta, \phi) \right].
\end{aligned} \tag{S11}$$

### Useful formula

The derivative of real spherical harmonics with respect to  $\theta$  requires to take the derivative of the associated Legendre polynomial  $P_l^m(\cos \theta)$ . This is given by:

$$\frac{\partial}{\partial \theta} P_l^m(\cos \theta) = \frac{1}{\sin \theta} [(l+1-m) P_{l+1}^m(\cos \theta) - (l+1) \cos \theta P_l^m(\cos \theta)] . \quad (\text{S12})$$

The derivative of real spherical harmonics with respect to  $\phi$  depends on  $m$  as follows:

$$\frac{\partial}{\partial \phi} Y_m^l(\theta, \phi) = \begin{cases} 0, & m = 0 \\ -m Y_{-m}^l(\theta, \phi), & m < 0 \\ -m Y_{-m}^l(\theta, \phi), & m > 0 \end{cases} . \quad (\text{S13})$$

When using GTOs as radial functions, the radial integrals are analytical:

$$\begin{aligned} I_{ln}^<(r) &= \int_0^r ds s^{2+l} R_n^l(s) \\ &= \mathcal{N}_{ln} \int_0^r ds s^{2+2l} \exp \left[ -\frac{1}{2} \left( \frac{s}{\sigma_{nl}} \right)^2 \right] \\ &= \mathcal{N}_{ln} 2^{\frac{1}{2}+l} \sigma_{nl}^{3+2l} \left\{ \Gamma \left[ \frac{3}{2} + l \right] - \Gamma \left[ \frac{3}{2} + l, \frac{1}{2} \left( \frac{r}{\sigma_{nl}} \right)^2 \right] \right\} \\ &= \mathcal{N}_{ln} 2^{\frac{1}{2}+l} \sigma_{nl}^{3+2l} \gamma \left[ \frac{3}{2} + l, \frac{1}{2} \left( \frac{r}{\sigma_{nl}} \right)^2 \right] , \end{aligned} \quad (\text{S14})$$

with  $\gamma$  the incomplete Gamma function, and

$$\begin{aligned} I_{ln}^>(r) &= \int_r^\infty ds s^{1-l} R_n^l(s) \\ &= \mathcal{N}_{ln} \int_r^\infty ds s \exp \left[ -\frac{1}{2} \left( \frac{s}{\sigma_{nl}} \right)^2 \right] \\ &= \mathcal{N}_{ln} \sigma_{nl}^2 \exp \left[ -\frac{1}{2} \left( \frac{r}{\sigma_{nl}} \right)^2 \right] , \end{aligned} \quad (\text{S15})$$

with the normalization factor given by

$$\mathcal{N}_{ln} = \sqrt{\frac{2}{\Gamma \left[ \frac{3}{2} + l \right] \sigma_{nl}^{3+2l}}} . \quad (\text{S16})$$

# DERIVATION OF HARTREE POTENTIAL AND ELECTRIC FIELD IN RECIPROCAL SPACE

Let us consider the Hartree potential that can be derived from the linear atom-centered expansion of the electron density  $n_e$  of a periodic system:

$$\begin{aligned}\phi_H(\mathbf{r}) &= \int_{\mathbf{R}^3} d\mathbf{r}' \frac{n_e(\mathbf{r}')}{|\mathbf{r} - \mathbf{r}'|} \\ &= \sum_{\mathbf{k} \neq \mathbf{0}} \frac{4\pi}{k^2} \tilde{n}_e(\mathbf{k}) e^{i\mathbf{k} \cdot \mathbf{r}} \\ &= \sum_{\mathbf{k} \neq \mathbf{0}}^{\text{half}} \frac{4\pi}{k^2} [\tilde{n}_e(\mathbf{k}) e^{i\mathbf{k} \cdot \mathbf{r}} + \tilde{n}_e(-\mathbf{k}) e^{-i\mathbf{k} \cdot \mathbf{r}}] .\end{aligned}\tag{S17}$$

The Fourier components of the electron density are given by

$$\begin{aligned}\tilde{n}_e(\mathbf{k}) &= \frac{1}{\Omega} \int_{\Omega} d\mathbf{r} e^{-i\mathbf{k} \cdot \mathbf{r}} n_e(\mathbf{r}) \\ &= \frac{1}{\Omega} \int_{\Omega} d\mathbf{r} e^{-i\mathbf{k} \cdot \mathbf{r}} \left[ \sum_{i, \mathbf{u}} \sum_{nlm} c_i^{nlm} R_n^l(|\mathbf{r} - \mathbf{r}_i - \mathbf{u}|) Y_m^l(\widehat{\mathbf{r} - \mathbf{r}_i - \mathbf{u}}) \right] \\ &= \frac{1}{\Omega} \sum_i e^{-i\mathbf{k} \cdot \mathbf{r}_i} \sum_{nlm} c_i^{nlm} \int_{\Omega} d\mathbf{s} e^{-i\mathbf{k} \cdot \mathbf{s}} \sum_{\mathbf{u}} [R_n^l(|\mathbf{s} - \mathbf{u}|) Y_m^l(\widehat{\mathbf{s} - \mathbf{u}})] \\ &= \frac{1}{\Omega} \sum_i e^{-i\mathbf{k} \cdot \mathbf{r}_i} \sum_{nlm} c_i^{nlm} \int_{\mathbf{R}^3} d\mathbf{s} e^{-i\mathbf{k} \cdot \mathbf{s}} R_n^l(s) Y_m^l(\hat{\mathbf{s}}) \\ &= \frac{1}{\Omega} \sum_i e^{-i\mathbf{k} \cdot \mathbf{r}_i} \sum_{nlm} c_i^{nlm} \int_{\mathbf{R}^3} d\mathbf{s} \left[ 4\pi \sum_{lm} (-i)^l j_l(ks) Y_m^l(\hat{\mathbf{k}}) Y_m^{l*}(\hat{\mathbf{s}}) \right] R_n^l(s) Y_m^l(\hat{\mathbf{s}}) \\ &= \frac{4\pi}{\Omega} \sum_i e^{-i\mathbf{k} \cdot \mathbf{r}_i} \sum_{nlm} c_i^{nlm} (-i)^l Y_m^l(\hat{\mathbf{k}}) \int_0^\infty ds s^2 j_l(ks) R_n^l(s) \\ &= \frac{4\pi}{\Omega} \sum_i e^{-i\mathbf{k} \cdot \mathbf{r}_i} \sum_{nlm} c_i^{nlm} (-i)^l Y_m^l(\hat{\mathbf{k}}) I_{nl}(k) ,\end{aligned}\tag{S18}$$

with  $I_{nl}(k)$  the radial integrals. Upon plugging Eq. (S18) into Eq. (S17), we finally get

$$\begin{aligned}\phi_H(\mathbf{r}) &= \frac{16\pi^2}{\Omega} \sum_{\mathbf{k} \neq \mathbf{0}}^{\text{half}} \frac{1}{k^2} \sum_i \sum_{nlm} c_i^{nlm} (-i)^l I_{nl}(k) \left[ Y_m^l(\hat{\mathbf{k}}) e^{i\mathbf{k} \cdot (\mathbf{r} - \mathbf{r}_i)} + Y_m^l(-\hat{\mathbf{k}}) e^{-i\mathbf{k} \cdot (\mathbf{r} - \mathbf{r}_i)} \right] \\ &= \frac{16\pi^2}{\Omega} \sum_{\mathbf{k} \neq \mathbf{0}}^{\text{half}} \frac{1}{k^2} \sum_i \sum_{nlm} c_i^{nlm} (-i)^l I_{nl}(k) Y_m^l(\hat{\mathbf{k}}) \begin{cases} 2 \cos[\mathbf{k} \cdot (\mathbf{r} - \mathbf{r}_i)] , & l\%2 = 0 \\ 2i \sin[\mathbf{k} \cdot (\mathbf{r} - \mathbf{r}_i)] , & l\%2 \neq 0 \end{cases} \\ &= \frac{32\pi^2}{\Omega} \sum_{\mathbf{k} \neq \mathbf{0}}^{\text{half}} \frac{1}{k^2} \sum_i \sum_{nlm} c_i^{nlm} I_{nl}(k) Y_m^l(\hat{\mathbf{k}}) \begin{cases} (-1)^{\frac{l}{2}} \cos[\mathbf{k} \cdot (\mathbf{r} - \mathbf{r}_i)] , & l\%2 = 0 \\ (-1)^{\frac{l+3}{2}} \sin[\mathbf{k} \cdot (\mathbf{r} - \mathbf{r}_i)] , & l\%2 \neq 0 \end{cases} .\end{aligned}\tag{S19}$$

From this Equation, it is straightforward to compute the Hartree electric field  $\mathbf{E}_H(\mathbf{r}) = -\nabla \phi_H(\mathbf{r})$  as

$$\mathbf{E}_H(\mathbf{r}) = \frac{32\pi^2}{\Omega} \sum_{\mathbf{k} \neq \mathbf{0}}^{\text{half}} \frac{\mathbf{k}}{k^2} \sum_i \sum_{nlm} c_i^{nlm} I_{nl}(k) Y_m^l(\hat{\mathbf{k}}) \begin{cases} (-1)^{\frac{l}{2}} \sin[\mathbf{k} \cdot (\mathbf{r} - \mathbf{r}_i)] , & l\%2 = 0 \\ (-1)^{\frac{l+1}{2}} \cos[\mathbf{k} \cdot (\mathbf{r} - \mathbf{r}_i)] , & l\%2 \neq 0 \end{cases} .\tag{S20}$$

When GTOs are chosen as radial functions, the radial integrals can be analytically computed:

$$\begin{aligned}
I_{nl}(k) &= \int_0^\infty ds s^2 j_l(ks) R_{nl}(s) \\
&= \int_0^\infty ds s^2 j_l(ks) \left\{ \mathcal{N}_{nl} s^l \exp \left[ -\frac{1}{2} \left( \frac{s}{\sigma_{nl}} \right)^2 \right] \right\} \\
&= \mathcal{N}_{nl} \int_0^\infty ds s^{2+l} j_l(ks) \exp \left[ -\frac{1}{2} \left( \frac{s}{\sigma_{nl}} \right)^2 \right] \\
&= \frac{\sqrt{2}}{\Gamma^{\frac{1}{2}} \left[ l + \frac{3}{2} \right] \sigma_{ln}^{l+\frac{3}{2}}} \left\{ \sqrt{\frac{\pi}{2}} k^l \sigma_{ln}^{2(l+\frac{3}{2})} \exp \left[ -\frac{1}{2} (k \sigma_{nl})^2 \right] \right\} \\
&= \frac{\sqrt{\pi}}{\Gamma^{\frac{1}{2}} \left[ l + \frac{3}{2} \right]} k^l \sigma_{ln}^{(l+\frac{3}{2})} \exp \left[ -\frac{1}{2} (k \sigma_{nl})^2 \right],
\end{aligned} \tag{S21}$$

as obtained via Mathematica-13.0.

### Electric field implementation

In order to efficiently implement Eq. (S20), we rely on the following rewriting, that assumes that all atoms are of the same chemical species, and therefore are associated with the same type of basis functions:

$$\begin{aligned}
\mathbf{E}_H(\mathbf{r}) &= \frac{32\pi^2}{\Omega} \sum_{\mathbf{k} \neq \mathbf{0}}^{\text{half}} \frac{\mathbf{k}}{k^2} \sum_l \sum_i \left[ \sum_{nm} c_i^{nlm} I_{nl}(k) Y_m^l(\hat{\mathbf{k}}) \right] \begin{cases} (-1)^{\frac{l}{2}} \sin[\mathbf{k} \cdot (\mathbf{r} - \mathbf{r}_i)], & l \% 2 = 0 \\ (-1)^{\frac{l+1}{2}} \cos[\mathbf{k} \cdot (\mathbf{r} - \mathbf{r}_i)], & l \% 2 \neq 0 \end{cases} \\
&= \frac{32\pi^2}{\Omega} \sum_{\mathbf{k} \neq \mathbf{0}}^{\text{half}} \frac{\mathbf{k}}{k^2} \sum_l \sum_i G_i^l(\mathbf{k}) \begin{cases} (-1)^{\frac{l}{2}} \sin[\mathbf{k} \cdot (\mathbf{r} - \mathbf{r}_i)], & l \% 2 = 0 \\ (-1)^{\frac{l+1}{2}} \cos[\mathbf{k} \cdot (\mathbf{r} - \mathbf{r}_i)], & l \% 2 \neq 0 \end{cases} \\
&= \frac{32\pi^2}{\Omega} \sum_{\mathbf{k} \neq \mathbf{0}}^{\text{half}} \frac{\mathbf{k}}{k^2} \sum_l \begin{cases} (-1)^{\frac{l}{2}} \sum_i G_i^l(\mathbf{k}) \sin[\mathbf{k} \cdot (\mathbf{r} - \mathbf{r}_i)], & l \% 2 = 0 \\ (-1)^{\frac{l+1}{2}} \sum_i G_i^l(\mathbf{k}) \cos[\mathbf{k} \cdot (\mathbf{r} - \mathbf{r}_i)], & l \% 2 \neq 0 \end{cases} \\
&= \frac{32\pi^2}{\Omega} \sum_{\mathbf{k} \neq \mathbf{0}}^{\text{half}} \frac{\mathbf{k}}{k^2} \sum_l \begin{cases} (-1)^{\frac{l}{2}} \sum_i G_i^l(\mathbf{k}) [\sin(\mathbf{k} \cdot \mathbf{r}) \cos(\mathbf{k} \cdot \mathbf{r}_i) - \cos(\mathbf{k} \cdot \mathbf{r}) \sin(\mathbf{k} \cdot \mathbf{r}_i)], & l \% 2 = 0 \\ (-1)^{\frac{l+1}{2}} \sum_i G_i^l(\mathbf{k}) [\cos(\mathbf{k} \cdot \mathbf{r}) \cos(\mathbf{k} \cdot \mathbf{r}_i) + \sin(\mathbf{k} \cdot \mathbf{r}) \sin(\mathbf{k} \cdot \mathbf{r}_i)], & l \% 2 \neq 0 \end{cases} \\
&= \frac{32\pi^2}{\Omega} \sum_{\mathbf{k} \neq \mathbf{0}}^{\text{half}} \frac{\mathbf{k}}{k^2} \sum_l \begin{cases} (-1)^{\frac{l}{2}} [C_l(\mathbf{k}) \sin(\mathbf{k} \cdot \mathbf{r}) - S_l(\mathbf{k}) \cos(\mathbf{k} \cdot \mathbf{r})], & l \% 2 = 0 \\ (-1)^{\frac{l+1}{2}} [C_l(\mathbf{k}) \cos(\mathbf{k} \cdot \mathbf{r}) + S_l(\mathbf{k}) \sin(\mathbf{k} \cdot \mathbf{r})], & l \% 2 \neq 0 \end{cases}
\end{aligned} \tag{S22}$$

where the factors

$$\begin{cases} C_l(\mathbf{k}) = \sum_i G_i^l(\mathbf{k}) \cos(\mathbf{k} \cdot \mathbf{r}_i) = \sum_i \left[ \sum_{nm} c_i^{nlm} I_{nl}(k) Y_m^l(\hat{\mathbf{k}}) \right] \cos(\mathbf{k} \cdot \mathbf{r}_i) \\ S_l(\mathbf{k}) = \sum_i G_i^l(\mathbf{k}) \sin(\mathbf{k} \cdot \mathbf{r}_i) = \sum_i \left[ \sum_{nm} c_i^{nlm} I_{nl}(k) Y_m^l(\hat{\mathbf{k}}) \right] \sin(\mathbf{k} \cdot \mathbf{r}_i) \end{cases} \tag{S23}$$

can be precomputed to avoid performing the sum over atoms at each  $\mathbf{r}$ .

# EWALD SUMMATION METHOD IN A PERIODIC SYSTEM

The Hatree potential of a periodic system can be written in real space as

$$\phi_H(\mathbf{r}) = 4\pi \sum_i \sum_{nlm} \frac{c_i^{nlm}}{2l+1} \sum_{\mathbf{u}} Y_{lm}(\widehat{\mathbf{r} - \mathbf{r}_i - \mathbf{u}}) \left[ \frac{I_{nl}^<(|\mathbf{r} - \mathbf{r}_i - \mathbf{u}|)}{|\mathbf{r} - \mathbf{r}_i - \mathbf{u}|^{l+1}} + |\mathbf{r} - \mathbf{r}_i - \mathbf{u}|^l I_{nl}^>(|\mathbf{r} - \mathbf{r}_i - \mathbf{u}|) \right]. \quad (\text{S24})$$

In order for the sum over the periodic images of the atoms  $i$  to converge within a given cutoff distance  $r_{\text{cut}}$  from a given point  $\mathbf{r}$  in the unit cell, it is required that the radial part of the potential, namely the term in square parenthesis, decays sufficiently fast with  $r \equiv |\mathbf{r} - \mathbf{r}_i - \mathbf{u}|$ .  $I_{nl}^>$  decays super-exponentially with  $r$ , so that the corresponding term becomes quickly vanishing for increasing values of  $r$ . Conversely,  $I_{nl}^<$  saturates to a constant, e.g., as  $\text{erf}(r)$  for  $l = 0$ , so that the  $1/r^{l+1}$  term will determine a slowly-decaying behaviour at large  $r$ , which will make the potential slowly converging with  $\mathbf{u}$ .

To remedy this problem, we adopt the Ewald summation method and consider a new fictitious electron density  $n_e^{\text{ewald}}$  defined from the same density coefficients as the real density, and a new set of radial functions  $R_{ln}^{\text{ewald}}$ , i.e.,

$$R_{ln}^{\text{ewald}}(s) = \mathcal{N}_{nl}^{\text{ewald}} s^l \exp \left[ -\frac{1}{2} \left( \frac{s}{\sigma_{nl}^{\text{ewald}}} \right)^2 \right], \quad (\text{S25})$$

such that:

$$\int_0^\infty ds s^{2+l} R_{nl}^{\text{ewald}}(s) = \int_0^\infty ds s^{2+l} R_{nl}(s). \quad (\text{S26})$$

This choice constraints the normalization factor of  $R_{nl}^{\text{ewald}}$  as follows

$$\mathcal{N}_{nl}^{\text{ewald}} = \frac{\int_0^\infty ds s^{2+l} R_{nl}(s)}{\int_0^\infty ds s^{2+2l} \exp \left[ -\frac{1}{2} \left( \frac{s}{\sigma_{nl}^{\text{ewald}}} \right)^2 \right]} = \mathcal{N}_{nl} \left( \frac{\sigma_{nl}}{\sigma_{nl}^{\text{ewald}}} \right)^{3+2l}. \quad (\text{S27})$$

Then, we subtract the two densities as  $n_e - n_e^{\text{ewald}}$ , which allows us to redefine the radial integrals as

$$I_{ln}^<(r) = \int_0^r ds s^{2+l} [R_{nl}(s) - R_{nl}^{\text{ewald}}(s)] \quad (\text{S28})$$

and

$$I_{ln}^>(r) = \int_r^\infty ds s^{1-l} [R_{nl}(s) - R_{nl}^{\text{ewald}}(s)]. \quad (\text{S29})$$

When taking the limit of  $r \rightarrow \infty$ , the former radial integral is now also going to 0 with super-exponential rapidity, allowing us to efficiently converge the sum over periodic images in Eq. (S24) within a suitably chosen cutoff distance.

The missing term associated with the fictitious  $n_e^{\text{ewald}}$  density can be efficiently computed in plane waves for sufficiently large values of  $\sigma_{nl}^{\text{ewald}}$  and finally added to the real space contribution. In particular, the explicit formula

for the radial integral in reciprocal space, which makes use of the normalization constraint previously derived, becomes:

$$\begin{aligned}
I_{nl}(k) &= \int_0^\infty ds s^2 j_l(ks) R_{nl}^{\text{ewald}}(s) \\
&= \int_0^\infty ds s^2 j_l(ks) \left\{ \mathcal{N}_{nl}^{\text{ewald}} s^l \exp \left[ -\frac{1}{2} \left( \frac{s}{\sigma_{nl}^{\text{ewald}}} \right)^2 \right] \right\} \\
&= \mathcal{N}_{nl}^{\text{ewald}} \int_0^\infty ds s^{2+l} j_l(ks) \exp \left[ -\frac{1}{2} \left( \frac{s}{\sigma_{nl}^{\text{ewald}}} \right)^2 \right] \\
&= \mathcal{N}_{nl} \left( \frac{\sigma_{nl}}{\sigma_{nl}^{\text{ewald}}} \right)^{3+2l} \int_0^\infty ds s^{2+l} j_l(ks) \exp \left[ -\frac{1}{2} \left( \frac{s}{\sigma_{nl}^{\text{ewald}}} \right)^2 \right] \\
&= \frac{\sqrt{2}}{\Gamma^{\frac{1}{2}} \left[ l + \frac{3}{2} \right] \sigma_{ln}^{l+\frac{3}{2}}} \left( \frac{\sigma_{nl}}{\sigma_{nl}^{\text{ewald}}} \right)^{3+2l} \left\{ \sqrt{\frac{\pi}{2}} k^l (\sigma_{ln}^{\text{ewald}})^{3+2l} \exp \left[ -\frac{1}{2} (k \sigma_{nl}^{\text{ewald}})^2 \right] \right\} \\
&= \frac{\sqrt{\pi}}{\Gamma^{\frac{1}{2}} \left[ l + \frac{3}{2} \right]} k^l \sigma_{ln}^{(l+\frac{3}{2})} \exp \left[ -\frac{1}{2} (k \sigma_{nl}^{\text{ewald}})^2 \right].
\end{aligned} \tag{S30}$$

### Definition of the Ewald Gaussian widths

Following the same strategy as MetalWalls,  $\sigma_{nl}^{\text{ewald}}$  can be defined from the radial cutoff  $r_{\text{cut}}$  in real space, which is set as an input parameter. In particular, we would like to make sure that the slowest decaying radial terms in the real space contribution of the electrostatic potential, evaluated at  $r \equiv r_{\text{cut}}$ , are lower than a certain threshold  $\varepsilon$ , which is also set as an input parameter. After doing the math and incorporating in  $\varepsilon$  the inessential constants, the aforementioned inequality reads as follows:

$$\frac{1}{r_{\text{cut}}^{l+1}} 2^{\frac{1}{2}+l} \Gamma \left[ \frac{3}{2} + l, \frac{1}{2} \left( \frac{r_{\text{cut}}}{\sigma_{nl}^{\text{ewald}}} \right)^2 \right] - r_{\text{cut}}^l \left( \frac{1}{\sigma_{nl}^{\text{ewald}}} \right)^{1+2l} \exp \left[ -\frac{1}{2} \left( \frac{r_{\text{cut}}}{\sigma_{nl}^{\text{ewald}}} \right)^2 \right] < \varepsilon \tag{S31}$$

Checking against Mathematica-13.0, the leading order term of the expansion at  $r_{\text{cut}} \rightarrow \infty$  of the the incomplete  $\Gamma$ -function exactly cancels out with the second term, so that we are left with the following inequality, which holds at large cutoff values:

$$\frac{1}{r_{\text{cut}}^{2-l}} \exp \left[ -\frac{1}{2} \left( \frac{r_{\text{cut}}}{\sigma_{nl}^{\text{ewald}}} \right)^2 \right] < \varepsilon \tag{S32}$$

Note that  $\exp(-x^2)/x$  represents the leading order of the expansion of  $\text{erfc}(x)$  at  $x \rightarrow \infty$ , which immediately recovers the expression used in MetalWalls for  $l = 0$ . The angular dependence implies smaller Gaussian widths at increasing  $l$ , which however, is not practical to derive from the previous equation given that  $\varepsilon$  is not adimensional, and making it adimensional would yield an equation that cannot be explicitly solved for  $\sigma_{nl}^{\text{ewald}}$ . A more practical solution is to use the Ewald  $\sigma$ -value of MetalWalls all throughout and define the real-space cutoff for each angular momentum as  $r_{\text{cut}}^l \equiv 4 r_0^l$ , where  $r_0^l = \sigma \sqrt{2+l}$  is the distance at which  $r^2 R_l^{\text{ewald}}(r)$  attains its maximum. This choice has also the advantage of keeping the number of plane-waves constant when computing the reciprocal space contribution.

# TOTAL ELECTRIC FIELD AND PSEUDO-POTENTIAL TERM

It is instructive to compare the electric field arising from the electron density response to the electrolyte perturbations, and that associated with the full charge density.

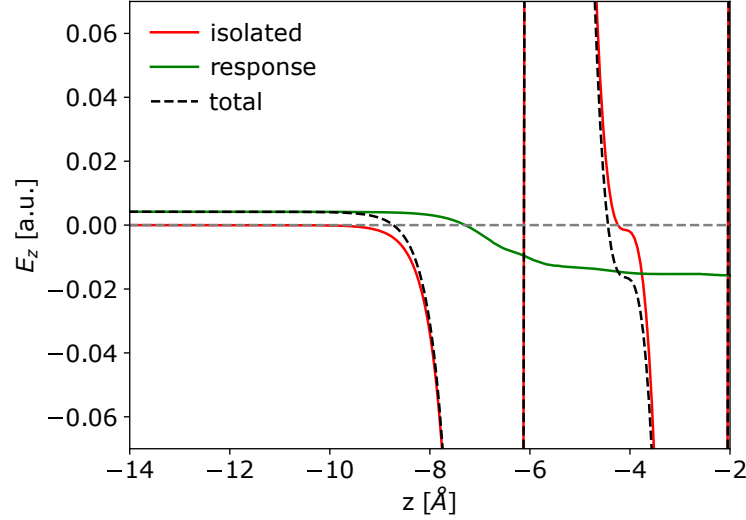

Figure S1: Kohn-Sham electric field at the electrochemical interface arising from the charge density response (green line), the total charge density (black dashed line), and the unperturbed total charge density (red line).

As shown in Fig. S1, while far from the electrode surface the response and the full charge density give rise to the same electric field, the electric field close to the surface varies massively in the two cases, implying that large differences are expected when the electrolyte atoms penetrate the electronic cloud of the electrode atoms, thus feeling the nuclear attraction. In case the electrode atoms are kept fixed, accounting for the full charge density requires to add to the response the contribution associated with the electron-density coefficients of the unperturbed electrode. In any case, the nuclear contribution to the electric field must also be added, which is associated with the classical part of the GTH pseudo-potentials used in CP2K [1]:

$$V_{\text{ion}}(r) = \frac{Z_{\text{eff}}}{r} \text{erf}\left(\frac{r}{\sqrt{2}r_{\text{loc}}}\right), \quad (\text{S33})$$

where  $Z_{\text{eff}} = 11$  and  $r_{\text{loc}} = 0.59065486855$  for the Au example reported in this work. Applying the Ewald summation method on this expression yields a short-range part computed in real space as:

$$V_{\text{ion}}^{\text{SR}}(r) = \frac{Z_{\text{eff}}}{r} \left[ \text{erf}\left(\frac{r}{\sqrt{2}r_{\text{loc}}}\right) - \text{erf}\left(\frac{r}{\sqrt{2}\sigma_{\text{ewald}}}\right) \right], \quad (\text{S34})$$

and a long-range part computed in reciprocal space as:

$$\tilde{V}_{\text{ion}}^{\text{LR}}(k) = \frac{4\pi}{\Omega} \frac{Z_{\text{eff}}}{k^2} \exp\left(-\frac{1}{2}k^2\sigma_{\text{ewald}}^2\right). \quad (\text{S35})$$

The short-range part of the electric field evaluated in a given point  $\mathbf{r}$  can be computed by relying on the same transformation matrix between Cartesian and spherical unit vectors already introduced. Considering that the angular components of the ionic potential are zero, we get:

$$\begin{aligned} \mathbf{E}_{\text{ion}}^{\text{SR}}(\mathbf{r}) &= -\nabla \sum_i V_{\text{ion}}^{\text{SR}}(|\mathbf{r} - \mathbf{r}_i|) \\ &= \sum_i \mathbf{U}(\mathbf{r} - \mathbf{r}_i) \cdot \left[ -\frac{\partial}{\partial r} V_{\text{ion}}^{\text{SR}}(r), 0, 0 \right] \end{aligned} \quad (\text{S36})$$

with

$$-\frac{\partial}{\partial r} V_{\text{ion}}^{\text{SR}}(r) = \frac{Z_{\text{eff}}}{r^2} \left[ \text{erf} \left( \frac{r}{\sqrt{2}r_{\text{loc}}} \right) - \text{erf} \left( \frac{r}{\sqrt{2}\sigma_{\text{ewald}}} \right) \right] - \sqrt{\frac{2}{\pi}} \left\{ \frac{Z_{\text{eff}}}{rr_{\text{loc}}} \exp \left[ -\frac{1}{2} \left( \frac{r}{r_{\text{loc}}} \right)^2 \right] - \frac{Z_{\text{eff}}}{r\sigma_{\text{ewald}}} \exp \left[ -\frac{1}{2} \left( \frac{r}{\sigma_{\text{ewald}}} \right)^2 \right] \right\} \quad (\text{S37})$$

The long-range part of the electric field evaluated in a given point  $\mathbf{r}$  is

$$\begin{aligned} \mathbf{E}_{\text{ion}}^{\text{LR}}(\mathbf{r}) &= -\nabla \left\{ 2 \sum_{\mathbf{k} \neq 0}^{\text{half}} \tilde{V}_{\text{ion}}^{\text{LR}}(k) \sum_i \cos[\mathbf{k} \cdot (\mathbf{r} - \mathbf{r}_i)] \right\} \\ &= \frac{8\pi}{\Omega} Z_{\text{eff}} \sum_{\mathbf{k} \neq 0}^{\text{half}} \frac{\mathbf{k}}{k^2} \exp \left( -\frac{1}{2} k^2 \sigma_{\text{ewald}}^2 \right) \sum_i \sin[\mathbf{k} \cdot (\mathbf{r} - \mathbf{r}_i)] \\ &= \frac{8\pi}{\Omega} Z_{\text{eff}} \sum_{\mathbf{k} \neq 0}^{\text{half}} \frac{\mathbf{k}}{k^2} \exp \left( -\frac{1}{2} k^2 \sigma_{\text{ewald}}^2 \right) \left[ \sin(\mathbf{k} \cdot \mathbf{r}) \sum_i \cos(\mathbf{k} \cdot \mathbf{r}_i) - \cos(\mathbf{k} \cdot \mathbf{r}) \sum_i \sin(\mathbf{k} \cdot \mathbf{r}_i) \right] \end{aligned} \quad (\text{S38})$$

where we used once again all the identities needed to perform an efficient calculation.

### LEARNING CURVES

We report here a learning curve associated with the SALTED electron density prediction computed over the test set used to validate the ML model, following the definition of percentage RMSE reported in the text.

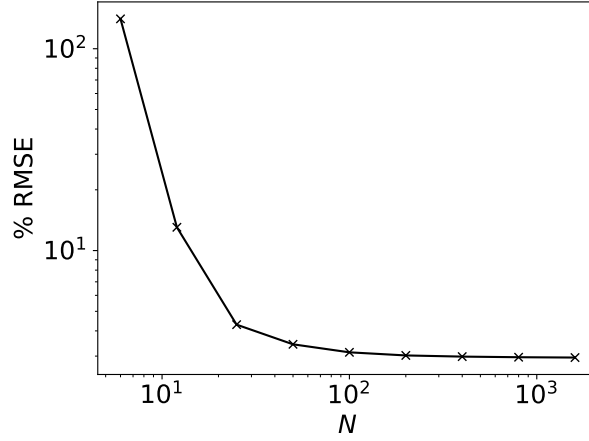

Figure S2: Learning curve reporting the % RMSE of the predicted electrode charge density of 400 randomly selected configurations, as a function of the training set size  $N$ .

# ANGULAR CORRELATION OF WATER MOLECULES

Fig. S3 shows the distribution of the dipole orientations of the first adsorption layers of water molecules with respect to the normal direction to the Au(100) surface, as computed from electrolyte configurations sampled every 1 ps over a total simulation time of 3 ns. Although smoother distribution functions would require to collect more statistics, we observe a noticeable difference between the SALTED and the classical simulation, consistently with the small classical prepeak of hydrogen atoms reported in the main text.

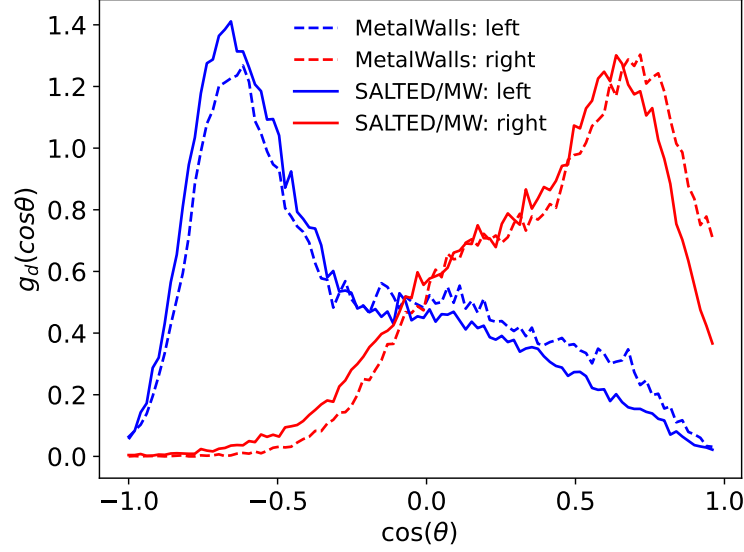

Figure S3: Angular distribution of water dipoles with respect to the normal direction to the electrode surface, for an applied potential of  $\Delta V = 1$  V. Blue and red lines refer to the first adsorption layers of water molecules on the left and right hand side of the gold electrode. Dashed lines: classical MetalWalls results. Full lines: SALTED/MetalWalls results.

---

\* andrea.grisafi@sorbonne-universite.fr

† mathieu.salanne@sorbonne-universite.fr

[S1] S. Goedecker, M. Teter, and J. Hutter. Separable dual-space gaussian pseudopotentials. *Phys. Rev. B*, 54:1703–1710, Jul 1996.
